# Supplementary material for: Block particle filters for state estimation of stochastic reaction-diffusion systems
Source: arXiv:2304.05392 source file (2023-04-07)
Supplement: Supplementary file 1 [file appendix.tex]

We assume that Eq.~\eqref{eq: Y_Process} describes how the signal of the state gets corrupted.    
Fig.~\ref{fig: measurements} shows simulated observations $y_k$ at single position $v = (v_1,v_2)$ for $k=1,\ldots,3000$. %Each $y_k$ consists of emissions at 10 different wavelengths $\lambda$. 

\begin{figure}[htb!] \centering
    \includegraphics[width=\columnwidth, scale=0.9]{figures/measurements}
    \vspace*{-1.5em}
    \caption{Observations at a random position $v$. }
    \label{fig: measurements}
\end{figure}
